# Supplementary material for: Three heats in strongly coupled system and bath
Source: arXiv:1810.13134 source file (2018-10-31)
Supplement: Supplementary file 1 [file 3heat_SM.pdf]

# Supplementary Material for nonequilibrium motion driven by a sliding harmonic potential

Chulan Kwon,[1] Jaegon Um,[2] Joonhyun Yeo,[3] and Hyunggyu Park[4]

[1]*Department of Physics, Myongji University, Yongin, Gyeonggi-Do, 17058, Korea*

[2]*BK21PLUS Physics Division, Pohang University of Science and Technology, Pohang 37673, Korea*

[3]*Department of Physics and Astronomy, Konkuk University, Seoul 08826, Korea*

[4]*School of Physics, Korea Institute for Advanced Study, Seoul 02455, Korea*

(Dated: today)

## I. MODEL

Equations of motion for a single colloid under a sliding harmonic potential and $N$ bath particles strongly coupled with the colloid are given as

$$\begin{aligned}
\dot{x} &= p/\mu \\
\dot{p} &= -k(x-ut) - \sum_{i=1}^{N} \kappa(x-x_i) \\
\dot{x}_i &= p_i/m \\
\dot{p}_i &= \gamma \frac{p_i}{m} - \kappa(x_i - x)
\end{aligned} \tag{1}$$

Using vector notations: $\mathbf{q}^* = (x-ut, p, x_1-ut, \cdots, x_i-ut, p_i, \cdots)^{\mathrm{t}}$, we can rewrite Eq. (1) as

$$\dot{\mathbf{q}}^* = -\mathsf{F}\cdot\mathbf{q}^* - \mathbf{u} + \boldsymbol{\xi}(t) \tag{2}$$

where

$$\mathsf{F} = \begin{bmatrix} 0 & -1/\mu & 0 & 0 & 0 & 0 & \cdots \\ k+N\kappa & 0 & -\kappa & 0 & -\kappa & 0 & \cdots \\ 0 & 0 & 0 & -1/m & 0 & 0 & \cdots \\ -\kappa & 0 & \kappa & \gamma/m & 0 & 0 & \cdots \\ 0 & 0 & 0 & 0 & 0 & -1/m & \cdots \\ -\kappa & 0 & 0 & 0 & \kappa & \gamma/m & \cdots \\ \cdots & \cdots & \cdots & \cdots & \cdots & \cdots & \cdots \end{bmatrix}, \quad \mathbf{u} = \begin{pmatrix} u \\ 0 \\ u \\ 0 \\ u \\ 0 \\ \vdots \end{pmatrix}, \quad \boldsymbol{\xi}(t) = \begin{pmatrix} 0 \\ 0 \\ 0 \\ \xi_1(t) \\ 0 \\ \xi_2(t) \\ \vdots \end{pmatrix} \tag{3}$$

The Hamiltonian at time $t$ is written as $(1/2)[p^2/\mu + k(x-ut)^2 + \sum_i (p_i^2/m) + \sum_i \kappa(x-x_i)^2]$, which is a function of $\mathbf{q}^*$ without explicit time dependence given as

$$H(\mathbf{q}^*) = \frac{1}{2}\mathbf{q}^*\cdot\mathsf{A}_{\mathrm{eq}}\cdot\mathbf{q}^* = \frac{1}{2}\mathbf{q}^*\cdot(\mathsf{A}_{\mathrm{S}} + \mathsf{A}_{\mathrm{I}} + \mathsf{A}_{\mathrm{B}})\cdot\mathbf{q}^*. \tag{4}$$

Here matrices are given as

$$\mathsf{A}_{\rm eq} = \begin{bmatrix} k+N\kappa & 0 & -\kappa & 0 & -\kappa & 0 & \cdots \\ 0 & 1/\mu & 0 & 0 & 0 & 0 & \cdots \\ -\kappa & 0 & \kappa & 0 & 0 & 0 & \cdots \\ 0 & 0 & 0 & 1/m & 0 & 0 & \cdots \\ -\kappa & 0 & 0 & 0 & \kappa & 0 & \cdots \\ 0 & 0 & 0 & 0 & 0 & 1/m & \cdots \\ \cdots & \cdots & \cdots & \cdots & \cdots & \cdots & \cdots \end{bmatrix}, \ \mathsf{A}_{\rm S} = \begin{bmatrix} k & 0 & 0 & 0 & 0 & 0 & \cdots \\ 0 & 1/\mu & 0 & 0 & 0 & 0 & \cdots \\ 0 & 0 & 0 & 0 & 0 & 0 & \cdots \\ 0 & 0 & 0 & 0 & 0 & 0 & \cdots \\ 0 & 0 & 0 & 0 & 0 & 0 & \cdots \\ 0 & 0 & 0 & 0 & 0 & 0 & \cdots \\ \cdots & \cdots & \cdots & \cdots & \cdots & \cdots & \cdots \end{bmatrix}$$

$$\mathsf{A}_{\rm I} = \begin{bmatrix} N\kappa & 0 & -\kappa & 0 & -\kappa & 0 & \cdots \\ 0 & 0 & 0 & 0 & 0 & 0 & \cdots \\ -\kappa & 0 & \kappa & 0 & 0 & 0 & \cdots \\ 0 & 0 & 0 & 0 & 0 & 0 & \cdots \\ -\kappa & 0 & 0 & 0 & \kappa & 0 & \cdots \\ 0 & 0 & 0 & 0 & 0 & 0 & \cdots \\ \cdots & \cdots & \cdots & \cdots & \cdots & \cdots & \cdots \end{bmatrix}, \ \mathsf{A}_{\rm B} = \begin{bmatrix} 0 & 0 & 0 & 0 & 0 & 0 & \cdots \\ 0 & 0 & 0 & 0 & 0 & 0 & \cdots \\ 0 & 0 & 0 & 0 & 0 & 0 & \cdots \\ 0 & 0 & 0 & 1/m & 0 & 0 & \cdots \\ 0 & 0 & 0 & 0 & 0 & 0 & \cdots \\ 0 & 0 & 0 & 0 & 0 & 1/m & \cdots \\ \cdots & \cdots & \cdots & \cdots & \cdots & \cdots & \cdots \end{bmatrix}, \tag{5}$$

We decompose $\mathbf{q}^* = \mathbf{z} + \mathbf{d}$, where the two parts independently satisfy the evolution equations as $\dot{\mathbf{d}} = -\mathsf{F}\cdot\mathbf{d} - \mathbf{u}$ and $\dot{\mathbf{z}} = -\mathsf{F}\cdot\mathbf{z} + \boldsymbol{\xi}(t)$. The deterministic part can be solved for initial condition $\mathbf{d}(0) = \mathsf{0}$ as $\mathbf{d}(t) = -\mathsf{F}^{-1}(\mathbf{I} - e^{-\mathsf{F}t})\cdot\mathbf{u}$. The probability density function (PDF) for the stochastic part $\mathbf{z}$ at time $t$ is known as

$$\sigma(\mathbf{z}, t) = \sqrt{\frac{|\beta \mathsf{A}_t|}{(2\pi)^d}} \exp\left[-\frac{\beta}{2}\mathbf{z}^{\rm t}\cdot\mathsf{A}_t\cdot\mathbf{z}\right] \tag{6}$$

where

$$\mathsf{A}_t^{-1} = \mathsf{A}_{\rm eq}^{-1} - \mathsf{U}_{t,0}\mathsf{A}_{\rm eq}^{-1}\mathsf{U}_{t,0}^{\rm t} + \mathsf{U}_{t,0}\mathsf{A}_0^{-1}\mathsf{U}_{t,0}^{\rm t} \tag{7}$$

for $\mathsf{U}_{t,t'} = e^{-\mathsf{F}(t-t')}$ and $\mathsf{U}_{t,t'}^{\rm t} = e^{-\mathsf{F}^{\rm t}(t-t')}$ for the superscription t denoting the transposition of matrix or vector. We numerically confirm $\mathsf{F}$ to be positive-definite, hence $e^{-\mathsf{F}t} \to \mathsf{0}$ for large $t$. For $\mathsf{A}_0 = \mathsf{A}_{\rm eq}$, $\mathsf{A}_t = \mathsf{A}_{\rm eq}$ at any time $t$. As $t$ goes large, $\mathsf{A}_t$ approaches $\mathsf{A}_{\rm eq}$, independent of intial condition. The PDF for $\mathbf{q}$ at $t$ is given by $\rho(\mathbf{q}, t) = \sigma(\mathbf{q} - \mathbf{u}t - \mathbf{d}(t), t)$. Nonequilibrium is characterized by nonzero mean of $\mathbf{q}$ equal to $\mathbf{u}t + \mathbf{d}(t)$, found from $\langle\mathbf{z}\rangle = \mathbf{0}$.

For a moving potential $U(x, t) = (k/2)(x - ut)^2$, we write the three heats and work

production accumulated for $0 < t < \tau$ as

$$W = \int_0^\tau dt \frac{\partial U(x,t)}{\partial t} = -ku \int_0^\tau dt[\mathbf{q}^*(t)]_x \quad (8)$$

$$Q_\alpha = W - \Delta \left[ \frac{1}{2} \mathbf{q}^* \cdot \mathsf{B}_\alpha \cdot \mathbf{q}^* \right] \quad (9)$$

where the subscript $x$ denotes the first (system-position) component of a vector and $\mathsf{B}_\alpha = \mathsf{A}_\mathrm{S}$, $\mathsf{A}_\mathrm{S} + \mathsf{A}_\mathrm{I}$, and $\mathsf{A}_\mathrm{eq}$, respectively for $\alpha = \mathrm{S},\ \mathrm{B},\ \mathrm{SB}$.

## II. INEQUALITIES FROM FLUCTUATION THEOREMS

In our model, any type (b) initial condition gives the divergence on the normalization condition because there is no constraint on the positions of bath particles. We consider a type (a) initial condition with $\mathsf{A}_0 = (\beta'/\beta)\mathsf{A}_\mathrm{S} + A_\mathrm{I} + \mathsf{A}_\mathrm{B}$ for which the system is in equilibrium with its own Hamilitonian $H_S(u=0)$ at an inverse temperature $\beta'$ and the bath is in an conditional equilibrium with the Hamiltonain $H_B + H_I$ at the inverse temperature $\beta$. Eq. (7) gives the kernel $\mathsf{A}_t$ at time $t$.

The reduced PDF is found as

$$\rho_\mathrm{S}(\mathbf{q}_S, t) = \frac{\sqrt{|\beta \mathsf{A}_{\mathrm{S},t}|}}{2\pi} \exp\left[ -\frac{\beta}{2} \mathbf{z}_\mathrm{S}(t)^\mathrm{t} \cdot \mathsf{A}_{\mathrm{S},t} \cdot \mathbf{z}_\mathrm{S}(t) \right] \quad (10)$$

where $[\mathsf{A}_{\mathrm{S},t}^{-1}]_{ij} = [\mathsf{A}_t^{-1}]_{ij}$ for $i,j = 1,2$ and $\mathbf{z}_\mathrm{S}(t) = \mathbf{q}_\mathrm{S} - \mathbf{u}_\mathrm{S} t - \mathbf{d}_\mathrm{S}(t)$ for $\mathbf{u}_\mathrm{S} = (u, 0)^\mathrm{t}$, $\mathbf{d}_\mathrm{S}(t) = (d_x(t), d_p(t))^\mathrm{t}$. Then, the average Shannon entropy change is given by

$$\langle -\Delta \ln \rho_\mathrm{S} \rangle = -\Delta \left[ \frac{1}{2} \ln \det \mathsf{A}_{\mathrm{S},t} - \frac{\beta}{2} \mathrm{Tr} \mathsf{A}_{\mathrm{S},t} \mathsf{A}_{\mathrm{S},t}^{-1} \right] = \frac{1}{2} \left[ \ln \det \mathsf{A}_{\mathrm{S},t}^{-1} - \ln \det \mathsf{A}_{\mathrm{S},0}^{-1} \right] \quad (11)$$

where we use the inverse matrix in the last step, which is easier to find directly from

$$\mathsf{A}_t^{-1} = \mathsf{A}_\mathrm{eq}^{-1} - \mathsf{U}_{t,0} \left[ \mathsf{A}_\mathrm{eq}^{-1} - ((\beta'/\beta)\mathsf{A}_\mathrm{S} + \mathsf{A}_\mathrm{I} + \mathsf{A}_\mathrm{B})^{-1} \right] \mathsf{U}_{t,0}^\mathrm{t}$$

The relative entropy change for type (a) is given as

$$\Delta D_\mathrm{a}(\rho || \tilde{\rho}) = \Delta \ln \left[ \frac{|\mathsf{A}_t|^{1/2} \exp\left[ -\frac{\beta}{2} \mathbf{z}(t)^\mathrm{t} \cdot \mathsf{A}_t \cdot \mathbf{z}(t) \right] \cdot |\mathsf{A}_{\mathrm{S},t}|^{-1/2} \exp\left[ \frac{\beta}{2} \mathbf{z}_\mathrm{S}(t)^\mathrm{t} \cdot \mathsf{A}_{\mathrm{S},t} \cdot \mathbf{z}_\mathrm{S}(t) \right]}{Z_\mathrm{B}^{-1} e^{\beta \tilde{H}_\mathrm{S}} \exp\left[ -\frac{\beta}{2} \mathbf{q}(t)^\mathrm{t} \cdot (\mathsf{A}_\mathrm{I} + \mathsf{A}_\mathrm{B}) \cdot \mathbf{q}(t) \right]} \right] \quad (12)$$

where $Z_\mathrm{B} = \mathrm{Tr}_\mathrm{B} e^{-\beta H_\mathrm{B}}$, and $e^{-\beta \tilde{H}_\mathrm{S}} = Z_\mathrm{B}^{-1} \mathrm{Tr}_\mathrm{B} e^{-\beta (H_\mathrm{B} + H_\mathrm{I})}$ is constant in our model. Its average vaue is found as

$$\begin{aligned} \langle \Delta D_\mathrm{a} \rangle = & \frac{1}{2} \left[ \ln \det \mathsf{A}_\tau^{-1} - \ln \det \mathsf{A}_0^{-1} \right] - \frac{1}{2} \left[ \ln \det \mathsf{A}_{\mathrm{S},\tau}^{-1} - \ln \det \mathsf{A}_{\mathrm{S},0}^{-1} \right] \\ & + \frac{\beta}{2} \mathrm{Tr}(\mathsf{A}_\tau^{-1} - \mathsf{A}_0^{-1})(\mathsf{A}_\mathrm{I} + \mathsf{A}_\mathrm{B}) + \frac{\beta}{2} (\mathbf{u}\tau + \mathbf{d}(\tau))^\mathrm{t} \cdot (\mathsf{A}_\mathrm{I} + \mathsf{A}_\mathrm{B}) \cdot (\mathbf{u}\tau + \mathbf{d}(\tau)) \ . \quad (13) \end{aligned}$$

The work $W$ accumulated for $0 < t \le \tau$ is equal to $\int_0^\tau dt(\partial/\partial t)(k/2)(x-ut)^2$. $x - ut = \mathbf{q}^*(t)_x = [\mathbf{d}(t) + \mathbf{z}(t)]_x$. Using $\langle \mathbf{z} \rangle = \mathbf{0}$ and $\mathbf{d}(t) = -\mathsf{F}^{-1}(1 - e^{-\mathsf{F}t}) \cdot \mathbf{u}$, its average value is found as

$$\begin{aligned}\langle W \rangle &= -ku \int_0^\tau \mathrm{d}t \mathbf{d}(t)_x \\ &= ku \int_0^\tau \mathrm{d}t [\mathsf{F}^{-1}(1 - e^{-\mathsf{F}t}) \cdot \mathbf{u}]_x = ku \left[ \mathsf{F}^{-1} \left( \tau - \mathsf{F}^{-1}(1 - e^{-\mathsf{F}\tau}) \right) \cdot \mathbf{u} \right]_x . \end{aligned} \tag{14}$$

Then, the average heat $Q_{\mathrm{S}}$ is found as

$$\begin{aligned}\langle Q_{\mathrm{S}} \rangle &= \langle W \rangle - \Delta \left\langle \frac{1}{2} \mathbf{q}^*(t)^{\mathrm{t}} \cdot \mathsf{A}_{\mathrm{S}} \cdot \mathbf{q}^*(t) \right\rangle \\ &= ku \left[ \mathsf{F}^{-1} \left( \tau - \mathsf{F}^{-1}(1 - e^{-\mathsf{F}\tau}) \right) \cdot \mathbf{u} \right]_x - \frac{1}{2} \mathbf{d}(\tau)^{\mathrm{t}} \cdot \mathsf{A}_{\mathrm{S}} \cdot \mathbf{d}(\tau) - \frac{1}{2} \mathrm{Tr} \mathsf{A}_{\mathrm{S}} (\mathsf{A}_\tau^{-1} - \mathsf{A}_0^{-1}). \end{aligned} \tag{15}$$

$\langle e^{\ln \rho_{\mathrm{S}} - \beta Q_{\mathrm{S}} + \Delta D_{\mathrm{a}}} \rangle = 1$ is independent of the inital condition and the $\langle e^{\ln \rho_{\mathrm{S}} - \beta Q_{\mathrm{S}}} \rangle = 1$ is derived for type (a) initial condition. In order to compare the inequalitities, $R_{\mathrm{a}} > 0$ and $R_{\mathrm{a}'} > 0$, we find

$$\begin{aligned} R_{\mathrm{a}} &= \langle -\ln \rho_{\mathrm{S}} \rangle + \beta \langle Q_{\mathrm{S}} \rangle - \langle \Delta D_{\mathrm{a}} \rangle \\ &= \frac{1}{2} \left[ \ln \det \mathsf{A}_\tau^{-1} - \ln \det \mathsf{A}_0^{-1} \right] - \frac{\beta}{2} \mathrm{Tr} \mathsf{A}_{\mathrm{eq}} (\mathsf{A}_\tau^{-1} - \mathsf{A}_0^{-1}) - \frac{\beta}{2} \mathbf{d}(\tau)^{\mathrm{t}} \cdot \mathsf{A}_{\mathrm{S}} \cdot \mathbf{d}(\tau) \\ &\quad + \beta ku \left[ \mathsf{F}^{-1} \left( \tau - \mathsf{F}^{-1}(1 - e^{-\mathsf{F}\tau}) \right) \cdot \mathbf{u} \right]_x - \frac{\beta}{2} (\mathbf{u}\tau + \mathbf{d}(\tau))^{\mathrm{t}} \cdot (\mathsf{A}_{\mathrm{I}} + \mathsf{A}_{\mathrm{B}}) \cdot (\mathbf{u}\tau + \mathbf{d}(\tau)), \end{aligned} \tag{16}$$

$$\begin{aligned} R_{\mathrm{a}'} &= \langle -\ln \rho_{\mathrm{S}} \rangle + \beta \langle Q_{\mathrm{S}} \rangle \\ &= \frac{1}{2} \left[ \ln \det \mathsf{A}_{\mathrm{S},\tau}^{-1} - \ln \det \mathsf{A}_{\mathrm{S},0}^{-1} \right] - \frac{\beta}{2} \mathrm{Tr} \mathsf{A}_{\mathrm{S}} (\mathsf{A}_\tau^{-1} - \mathsf{A}_0^{-1}) - \frac{\beta}{2} \mathbf{d}(\tau)^{\mathrm{t}} \cdot \mathsf{A}_{\mathrm{S}} \cdot \mathbf{d}(\tau) \\ &\quad + \beta ku \left[ \mathsf{F}^{-1} \left( \tau - \mathsf{F}^{-1}(1 - e^{-\mathsf{F}\tau}) \right) \cdot \mathbf{u} \right]_x . \end{aligned} \tag{17}$$

## III. HEAT GENERATING FUNCTIONS

The generating function for heat $Q_\alpha$ is defined as $\mathcal{G}_\alpha(\lambda) = \langle e^{-\beta\lambda Q_\alpha} \rangle$ where $\langle \cdots \rangle$ denotes the average over all trajectories $\mathbf{z}(t)$ for $0 < t < \tau$, and intial and final states. We consider an intial condition with equilibrium PDF given by $\left[ \det \beta \mathsf{A}_{\mathrm{eq}} / (2\pi)^d \right]^{1/2} \exp\left[ -\frac{\beta}{2} \mathbf{z}_0^{\mathrm{t}} \cdot \mathsf{A}_{\mathrm{eq}} \cdot \mathbf{z}_0 \right]$

for $d=2(N+1)$. We have

$$
\begin{aligned}
\mathcal{G}_\alpha(\lambda) &= \int \mathrm{d}\mathbf{z}_\tau \exp\left[\frac{\beta\lambda}{2}\mathbf{q}_\tau^{*\mathrm{t}}\cdot\mathsf{B}_\alpha\cdot\mathbf{q}_\tau^*\right]\int \mathrm{d}\mathbf{z}_0 \int \mathrm{D}[\mathbf{z}(t)]\ \Pi[\mathbf{z}(t);\mathbf{z}_\tau,\mathbf{z}_0]\exp\left[\beta\lambda k u\int_0^\tau \mathrm{d}t[\mathbf{q}^*(t)]_x\right] \\
&\quad\times\exp\left[-\frac{\beta\lambda}{2}\mathbf{q}_0^{*\mathrm{t}}\cdot\mathsf{B}_\alpha\cdot\mathbf{q}_0^*\right]\left[\frac{\det\beta\mathsf{A}_{\mathrm{eq}}}{(2\pi)^d}\right]^{1/2}\exp\left[-\frac{\beta}{2}\mathbf{z}_0^{\mathrm{t}}\cdot\mathsf{A}_{\mathrm{eq}}\cdot\mathbf{z}_0\right] \\
&= \left[\frac{\det\mathsf{A}_{\mathrm{eq}}}{\det(\mathsf{A}_{\mathrm{eq}}+\lambda\mathsf{B}_\alpha)}\right]^{1/2}\int \mathrm{d}\mathbf{z}_\tau\exp\left[\frac{\beta\lambda}{2}\mathbf{q}_\tau^{*\mathrm{t}}\cdot\mathsf{B}_\alpha\cdot\mathbf{q}_\tau^*\right]\int \mathrm{d}\mathbf{z}_0\int \mathrm{D}[\mathbf{z}(t)]\ \Pi[\mathbf{z}(t);\mathbf{z}_\tau,\mathbf{z}_0] \\
&\quad\times\exp\left[\beta\lambda k u\int_0^\tau \mathrm{d}t[\mathbf{q}^*(t)]_x\right]\ \left[\frac{\det\beta(\mathsf{A}_{\mathrm{eq}}+\lambda\mathsf{B}_\alpha)}{(2\pi)^d}\right]^{1/2}\exp\left[-\frac{\beta}{2}\mathbf{z}_0^{\mathrm{t}}\cdot(\mathsf{A}_{\mathrm{eq}}+\lambda\mathsf{B}_\alpha)\cdot\mathbf{z}_0\right] \\
&= \left[\frac{\det\mathsf{A}_{\mathrm{eq}}\det\mathsf{A}_{\tau,\lambda}}{\det(\mathsf{A}_{\mathrm{eq}}+\lambda\mathsf{B}_\alpha)\det(\mathsf{A}_{\tau,\lambda}-\lambda\mathsf{B}_\alpha)}\right]^{1/2}\int \mathrm{d}\mathbf{z}_\tau\left[\frac{\det(\mathsf{A}_{\tau,\lambda}-\lambda\mathsf{B}_\alpha)}{\det\mathsf{A}_{\tau,\lambda}}\right]^{1/2}\exp\left[\frac{\beta\lambda}{2}\mathbf{q}_\tau^{*\mathrm{t}}\cdot\mathsf{B}_\alpha\cdot\mathbf{q}_\tau^*\right] \\
&\quad\times\int \mathrm{d}\mathbf{z}_0\int \mathrm{D}[\mathbf{z}(t)]\ \Pi[\mathbf{z}(t);\mathbf{z}_\tau,\mathbf{z}_0]\exp\left[\beta\lambda k u\int_0^\tau \mathrm{d}t[\mathbf{q}^*(t)]_x\right] \\
&\quad\times\left[\frac{\det\beta(\mathsf{A}_{\mathrm{eq}}+\lambda\mathsf{B}_\alpha)}{(2\pi)^d}\right]^{1/2}\exp\left[-\frac{\beta}{2}\mathbf{z}_0^{\mathrm{t}}\cdot(\mathsf{A}_{\mathrm{eq}}+\lambda\mathsf{B}_\alpha)\cdot\mathbf{z}_0\right] \\
&= N_\alpha c_\alpha\left\langle\exp\left[\beta\lambda\mathbf{d}_\tau^{\mathrm{t}}\cdot\mathsf{B}_\alpha\cdot\mathbf{z}_\tau+\beta\lambda k u\int_0^\tau \mathrm{d}t[\mathbf{z}(t)]_x\right]\right\rangle_{\mathrm{ren}}
\end{aligned}
\tag{18}
$$

where $\Pi[\mathbf{z}(t);\mathbf{z}_\tau,\mathbf{z}_0]$ is the probability for path $\mathbf{z}(t)$ connecting $\mathbf{z}_0$ at $t=0$ and $\mathbf{z}_\tau$ at $t=\tau$. $\langle\cdots\rangle_{\mathrm{ren}}$ is the renormalized integration with altered initial and final PDF given as

$$
\begin{aligned}
\sigma(\mathbf{z}_0,0) &= \left[\frac{\det\beta(\mathsf{A}_{\mathrm{eq}}+\lambda\mathsf{B}_\alpha)}{(2\pi)^d}\right]^{1/2}\exp\left[-\frac{\beta}{2}\mathbf{z}_0^{\mathrm{t}}\cdot(\mathsf{A}_{\mathrm{eq}}+\lambda\mathsf{B}_\alpha)\cdot\mathbf{z}_0\right] \\
\sigma(\mathbf{z}_\tau,\tau) &= \left[\frac{\det\beta(\mathsf{A}_{\tau,\lambda}-\lambda\mathsf{B}_\alpha)}{(2\pi)^d}\right]^{1/2}\exp\left[-\frac{\beta}{2}\mathbf{z}_\tau^{\mathrm{t}}\cdot(\mathsf{A}_{\tau,\lambda}-\lambda\mathsf{B}_\alpha)\cdot\mathbf{z}_\tau\right]\ ,
\end{aligned}
\tag{19}
$$

where, similarly to Eq. (7),

$$
\mathsf{A}_{\tau,\lambda}^{-1}=\mathsf{A}_{\mathrm{eq}}^{-1}-\mathsf{U}_{t,0}\mathsf{A}_{\mathrm{eq}}^{-1}\mathsf{U}_{t,0}^{\mathrm{t}}+\mathsf{U}_{t,0}(\mathsf{A}_{\mathrm{eq}}+\lambda\mathsf{B}_\alpha)\mathsf{U}_{t,0}^{\mathrm{t}}
\tag{20}
$$

The renormalization constant is given as

$$
N_\alpha=\left[\frac{\det\mathsf{A}_{\mathrm{eq}}\det\mathsf{A}_{\tau,\lambda}}{\det(\mathsf{A}_{\mathrm{eq}}+\lambda\mathsf{B}_\alpha)\det(\mathsf{A}_{\tau,\lambda}-\lambda\mathsf{B}_\alpha)}\right]^{1/2}.
\tag{21}
$$

$c_\alpha$ is the coefficient independent of the integration, which is given using $\mathbf{q}_\tau^*=\mathbf{z}_\tau+\mathbf{d}_\tau$ as

$$
c_\alpha=\exp\left[\frac{\beta\lambda}{2}\mathbf{d}_\tau^{\mathrm{t}}\cdot\mathsf{B}_\alpha\cdot\mathbf{d}_\tau+\beta\lambda k u\int_0^\tau \mathrm{d}t[\mathbf{d}(t)]_x\right]
\tag{22}
$$

where $\mathbf{d}(t)=-\mathsf{F}^{-1}(1-e^{-\mathsf{F}t})\cdot\mathbf{u}$ is used.

$\langle\cdots\rangle_{\rm ren}$ in Eq. (18) can be evaluated by using the cumulant expansion as

$$f_\alpha = \exp\left[\frac{(\beta\lambda)^2}{2}\mathbf{d}_\tau^{\rm t}\cdot\mathsf{B}_\alpha\tilde{\mathsf{C}}_\alpha(\tau,\tau)\mathsf{B}_\alpha\cdot\mathbf{d}_\tau + \frac{(\beta\lambda ku)^2}{2}\int_0^\tau {\rm d}t\int_0^\tau {\rm d}t'[\tilde{\mathsf{C}}_\alpha]_{xx}(t,t') \right.$$
$$\left. +(\beta\lambda)^2 ku\int_0^\tau {\rm d}t\left[\mathbf{d}_\tau^{\rm t}\cdot\mathsf{B}_\alpha\tilde{\mathsf{C}}_\alpha(\tau,t)\right]_x\right] \ , \qquad (23)$$

where $\tilde{C}_\alpha(t,t') = \langle\mathbf{z}(t)\mathbf{z}^{\rm t}(t')\rangle_{\rm ren}$ is a renormalized correlation function matrix, which is different for each type $\alpha$. It can be found from

$$\left\langle\exp\left[\mathbf{l}_1^{\rm t}\cdot\mathbf{z}(t_1)+\mathbf{l}_2^{\rm t}\cdot\mathbf{z}(t_2)\right]\right\rangle_{\rm ren} = \left\langle\exp\left[(1/2)\sum_{i,j}\mathbf{l}_i^{\rm t}\cdot\tilde{C}(t_i,t_j)\cdot\mathbf{l}_j\right]\right\rangle_{\rm ren} \ . \qquad (24)$$

We have

$$\left\langle\exp\left[\mathbf{l}_1^{\rm t}\cdot\mathbf{z}(t_1)+\mathbf{l}_2^{\rm t}\cdot\mathbf{z}(t_2)\right]\right\rangle_{\rm ren}$$
$$=\int {\rm d}\mathbf{z}_\tau\left[\frac{\det(\mathsf{A}_{\tau,\lambda}-\lambda\mathsf{B}_\alpha)}{\det\mathsf{A}_{\tau,\lambda}}\right]^{1/2}\exp\left[\frac{\beta\lambda}{2}\mathbf{z}_\tau^{\rm t}\cdot\mathsf{B}_\alpha\cdot\mathbf{z}_\tau\right]\int {\rm d}\mathbf{z}_1 T[\mathbf{z}_\tau,\tau;\mathbf{z}_1,t_1]\exp\left[\mathbf{l}_1\cdot\mathbf{z}_1\right]$$
$$\times\int {\rm d}\mathbf{z}_2 T[\mathbf{z}_1,t_1;\mathbf{z}_2,t_2]\left[\frac{\det\beta\mathsf{A}_{t_2,\lambda}}{(2\pi)^d}\right]^{1/2}\exp\left[-\frac{\beta}{2}\mathbf{z}_2^{\rm t}\cdot\mathsf{A}_{t_2,\lambda}\cdot\mathbf{z}_2+\mathbf{l}_2\cdot\mathbf{z}_2\right] \ , \qquad (25)$$

Here the propagator for the transition from $\mathbf{z}_2$ at $t_2$ to $\mathbf{z}_1$ at $t_1$, defined as $\int {\rm D}\mathbf{z}(t)\Pi[\mathbf{z}(t);\mathbf{z}_1,\mathbf{z}_2]$, is given as

$$T[\mathbf{z}_1,t_1;\mathbf{z}_2,t_2] = \left[\frac{\det\beta\mathsf{A}_{t_i,t_2}}{(2\pi)^d}\right]^{1/2}\exp\left[-\frac{\beta}{2}(\mathbf{z}_1-\mathsf{U}_{t_1,t_2}\cdot\mathbf{z}_2)^{\rm t}\cdot\mathsf{A}_{t_1,t_2}\cdot(\mathbf{z}_1-\mathsf{U}_{t_1,t_2}\cdot\mathbf{z}_2)\right] \ , \qquad (26)$$

where

$$\mathsf{A}_{t_1,t_2}^{-1} = \mathsf{A}_{\rm eq}^{-1} - \mathsf{U}_{t_1,t_2}\mathsf{A}_{\rm eq}^{-1}\mathsf{U}_{t_1,t_2}^{\rm t}. \qquad (27)$$

Eqs. (7), (20), (27) are similar, but different by initial condition. Eq. (25) can be found by carrying out integrations repeatedly and the renormalized correlation function matrix is found as for $t > t'$

$$\tilde{\mathsf{C}}_\alpha(t,t') = \beta^{-1}\mathsf{U}_{t,t'}\mathsf{A}_{t',\lambda}^{-1} + \beta^{-1}\mathsf{A}_{t,\lambda}^{-1}\mathsf{U}_{\tau,t}^{\rm t}\mathsf{A}_{\tau,\lambda}\left[(\mathsf{A}_{\tau,\lambda}-\lambda\mathsf{B}_\alpha)^{-1}-\mathsf{A}_{\tau,\lambda}^{-1}\right]\mathsf{A}_{\tau,\lambda}\mathsf{U}_{\tau,t'}\mathsf{A}_{t',\lambda}^{-1} \ . \qquad (28)$$

For $\lambda = 0$, $\mathsf{A}_{t,\lambda} = \mathsf{A}_t$ and $\tilde{\mathsf{A}}(t,t') = \beta^{-1}e^{-\mathsf{F}(t-t')}\mathsf{A}_{t'}^{-1}$ becomes the usual correlation function.

As a result, we have the generating function for each type $\alpha$ as

$$
\begin{aligned}
\mathcal{G}_\alpha(\lambda) &= N_\alpha c_\alpha f_\alpha(\lambda) \\
&= \left[\frac{\det \mathsf{A}_{\rm eq} \det \mathsf{A}_{\tau,\lambda}}{\det(\mathsf{A}_{\rm eq}+\lambda \mathsf{B}_\alpha)\det(\mathsf{A}_{\tau,\lambda}-\lambda\mathsf{B}_\alpha)}\right]^{1/2} \\
&\quad \times \exp\left[\frac{(\beta\lambda)^2}{2}\mathbf{d}_\tau^{\rm t}\cdot \mathsf{B}_\alpha \tilde{\mathsf{C}}_\alpha(\tau,\tau)\mathsf{B}_\alpha\cdot\mathbf{d}_\tau + \frac{(\beta\lambda k u)^2}{2}\int_0^\tau {\rm d}t \int_0^\tau {\rm d}t' [\tilde{\mathsf{C}}_\alpha]_{xx}(t,t') \right.\\
&\quad \left. +(\beta\lambda)^2 k u \int_0^\tau {\rm d}t \left[\mathbf{d}_\tau^{\rm t}\cdot \mathsf{B}_\alpha\tilde{\mathsf{C}}_\alpha(\tau,t)\right]_x\right] \\
&\quad \times \exp\left[\frac{(\beta\lambda)^2}{2}\mathbf{d}_\tau^{\rm t}\cdot \mathsf{B}_\alpha \tilde{\mathsf{C}}_\alpha(\tau,\tau)\mathsf{B}_\alpha\cdot\mathbf{d}_\tau + \frac{(\beta\lambda k u)^2}{2}\int_0^\tau {\rm d}t \int_0^\tau {\rm d}t' [\tilde{\mathsf{C}}_\alpha]_{xx}(t,t') \right.\\
&\quad \left. +(\beta\lambda)^2 k u \int_0^\tau {\rm d}t \left[\mathbf{d}_\tau^{\rm t}\cdot \mathsf{B}_\alpha\tilde{\mathsf{C}}_\alpha(\tau,t)\right]_x\right] .
\end{aligned} \tag{29}
$$

## IV. HEAT GENERATING FUNCTIONS FOR LONG TIME

We will find the functions, $\mathcal{G}_\alpha(\lambda) = N_\alpha c_\alpha f_\alpha$, for heats accumulated for long time $\tau$ where $e^{-\mathsf{F}\tau}$ can be neglected. $\mathsf{A}_{\tau,\lambda}$ in Eq. (20) is complicated due to the initial condition: $\mathsf{A}_{0,\lambda} = (\mathsf{A}_{\rm eq}+\lambda\mathsf{B}_\alpha)^{-1}$. However, for large $\tau$, we have $\mathsf{A}_{\tau,\lambda}\simeq \mathsf{A}_{\rm eq}$.

We first find $N_\alpha$ as

$$
N_\alpha = \left[\frac{|\det \mathsf{A}_{\rm eq}|^2}{\det(\mathsf{A}_{\rm eq}+\lambda\mathsf{B}_\alpha)\det(\mathsf{A}_{\rm eq}-\lambda\mathsf{B}_\alpha)}\right]^{1/2} = \frac{1}{(1-\lambda^2)^\nu} \quad \text{for } \nu = \begin{cases} 1 & \alpha = {\rm S} \\ N/2+1 & \alpha = {\rm B} \\ N+1 & \alpha = {\rm SB} \end{cases} . \tag{30}
$$

Next, we find $c_\alpha$ in Eq. (22) as

$$
c_\alpha = \exp\left[\frac{\beta\lambda}{2}\mathbf{u}^{\rm t}\cdot(\mathsf{F}^{\rm t})^{-1}\mathsf{B}_\alpha\mathsf{F}^{-1}\cdot\mathbf{u} - \beta\lambda k u\left(\left[\mathsf{F}^{-1}\cdot\mathbf{u}\right]_x\tau - \left[\mathsf{F}^{-2}\cdot\mathbf{u}\right]_x\right)\right]. \tag{31}
$$

$f_\alpha$ in Eq. (23) is much complicated, given as

$$
\begin{aligned}
f_\alpha = \exp\Bigg[&\frac{(\beta\lambda)^2}{2}\mathbf{u}^{\rm t}\cdot(\mathsf{F}^{\rm t})^{-1}\mathsf{B}_\alpha(\mathsf{I}-\lambda\mathsf{A}_{\rm eq}^{-1}\mathsf{B}_\alpha)^{-1}\mathsf{A}_{\rm eq}^{-1}\mathsf{B}_\alpha\mathsf{F}^{-1}\cdot\mathbf{u} \\
&+(\beta\lambda)^2 k u \underbrace{\int_0^\tau {\rm d}t[\mathbf{d}_\tau^{\rm t}\cdot\mathsf{B}_\alpha\tilde{\mathsf{C}}_\alpha(\tau,t)]_x}_{I_{\alpha 1}} + \frac{(\beta\lambda k u)^2}{2}\underbrace{\int_0^\tau {\rm d}t\int_0^\tau {\rm d}t'[\tilde{\mathsf{C}}_\alpha(t,t')]_{xx}}_{I_{\alpha 2}}\Bigg] ,
\end{aligned} \tag{32}
$$

where the integrals in the last two terms are complicated to evaluate. Using $\mathsf{A}_{\tau,\lambda} = \mathsf{A}_{\rm eq}$ for

large $\tau$, $\tilde{C}_\alpha(t,t')$ for $t > t'$ is given in more detail as

$$\begin{aligned}
\tilde{C}_\alpha(t,t') &= \beta^{-1} e^{-\mathsf{F}t}\left[e^{\mathsf{F}t'}\mathsf{A}_{\mathrm{eq}}^{-1} - \lambda \mathsf{A}_{\mathrm{eq}}^{-1}(\mathsf{I}+\lambda\mathsf{B}_\alpha\mathsf{A}_{\mathrm{eq}}^{-1})^{-1}\mathsf{B}_\alpha\mathsf{A}_{\mathrm{eq}}^{-1}e^{-\mathsf{F}^{\mathrm{t}}t'}\right] \\
&+ \beta^{-1}\lambda\left[\mathsf{A}_{\mathrm{eq}}^{-1}e^{\mathsf{F}^{\mathrm{t}}t} - e^{-\mathsf{F}t}\mathsf{A}_{\mathrm{eq}}^{-1}(\mathsf{I}+\lambda\mathsf{B}_\alpha\mathsf{A}_{\mathrm{eq}}^{-1})^{-1}\mathsf{B}_\alpha\mathsf{A}_{\mathrm{eq}}^{-1}\right]e^{-\mathsf{F}^{\mathrm{t}}\tau}\mathsf{A}_{\mathrm{eq}}\left[\mathsf{I}-\lambda\mathsf{A}_{\mathrm{eq}}^{-1}\mathsf{B}_\alpha\right]^{-1}\mathsf{A}_{\mathrm{eq}}^{-1}\mathsf{B}_\alpha \\
&\times e^{-\mathsf{F}\tau}\left[e^{\mathsf{F}t'}\mathsf{A}_{\mathrm{eq}}^{-1} - \mathsf{A}_{\mathrm{eq}}^{-1}(\mathsf{I}+\lambda\mathsf{B}_\alpha\mathsf{A}_{\mathrm{eq}}^{-1})^{-1}\mathsf{B}_\alpha\mathsf{A}_{\mathrm{eq}}^{-1}e^{-\mathsf{F}^{\mathrm{t}}t'}\right] \ . \qquad (33)
\end{aligned}$$

Then, we find

$$\begin{aligned}
I_{\alpha 1} &= -\beta^{-1}\int_0^\tau \mathrm{d}t\mathbf{u}^{\mathrm{t}}\cdot(\mathsf{F}^{-1})^{\mathrm{t}}\mathsf{B}_\alpha(\mathsf{I}-\lambda\mathsf{A}_{\mathrm{eq}}^{-1}\mathsf{B}_\alpha)^{-1}e^{-\mathsf{F}(\tau-t)}\mathsf{A}_{\mathrm{eq}}^{-1} + \mathcal{O}(e^{-\mathsf{F}\tau}) \\
&= -\beta^{-1}\mathbf{u}^{\mathrm{t}}\cdot(\mathsf{F}^{-1})^{\mathrm{t}}\mathsf{B}_\alpha(\mathsf{I}-\lambda\mathsf{A}_{\mathrm{eq}}^{-1}\mathsf{B}_\alpha)^{-1}\mathsf{F}^{-1}\mathsf{A}_{\mathrm{eq}}^{-1} + \mathcal{O}(e^{-\mathsf{F}\tau}) \ . \qquad (34)
\end{aligned}$$

We write

$$\mathsf{S}_\alpha^+ = (\mathsf{I}+\lambda\mathsf{B}_\alpha\mathsf{A}_{\mathrm{eq}}^{-1})^{-1}\mathsf{B}_\alpha\mathsf{A}_{\mathrm{eq}}^{-1} \ , \quad \mathsf{S}_\alpha^- = \left[\mathsf{I}-\lambda\mathsf{A}_{\mathrm{eq}}^{-1}\mathsf{B}_\alpha\right]^{-1}\mathsf{A}_{\mathrm{eq}}^{-1}\mathsf{B}_\alpha \ , \qquad (35)$$

which turn out to be $(1+\lambda)^{-1}$ and $(1-\lambda)^{-1}$, respectively. Then, we find

$$\begin{aligned}
I_{\alpha 2} &= 2\int_0^\tau \mathrm{dt}\int_0^t \mathrm{d}t'\tilde{C}_\alpha(t,t') \\
&= 2\beta^{-1}\int_0^\tau \mathrm{d}t\left[\mathsf{F}^{-1}(1-e^{-\mathsf{F}t})\mathsf{A}_{\mathrm{eq}}^{-1} + \lambda e^{-\mathsf{F}t}\mathsf{A}_{\mathrm{eq}}^{-1}\mathsf{S}_\alpha^+(\mathsf{F}^{\mathrm{t}})^{-1}(e^{-\mathsf{F}^{\mathrm{t}}t}-1)\right] \\
&\quad +2\beta^{-1}\lambda\int_0^\tau \mathrm{d}t\mathsf{A}_{\mathrm{eq}}^{-1}e^{-\mathsf{F}^{\mathrm{t}}(\tau-t)}\mathsf{A}_{\mathrm{eq}}\mathsf{S}_\alpha^-\mathsf{F}^{-1}e^{-\mathsf{F}(\tau-t)}\mathsf{A}_{\mathrm{eq}}^{-1} + \mathcal{O}(e^{-\mathsf{F}t}) \\
&= 2\beta^{-1}\Big[\mathsf{F}^{-1}(\tau-\mathsf{F}^{-1})\mathsf{A}_{\mathrm{eq}}^{-1} - \lambda\mathsf{F}^{-1}\mathsf{A}_{\mathrm{eq}}^{-1}\mathsf{S}_\alpha^+(\mathsf{F}^{\mathrm{t}})^{-1} \\
&\quad +\lambda\int_0^\tau \mathrm{d}te^{-\mathsf{F}t}\mathsf{A}_{\mathrm{eq}}^{-1}\mathsf{S}_\alpha^+(\mathsf{F}^{\mathrm{t}})^{-1}e^{-\mathsf{F}^{\mathrm{t}}t} + \lambda\int_0^\tau \mathrm{d}t\mathsf{A}_{\mathrm{eq}}^{-1}e^{-\mathsf{F}^{\mathrm{t}}t}\mathsf{A}_{\mathrm{eq}}\mathsf{S}_\alpha^-\mathsf{F}^{-1}e^{-\mathsf{F}t}\mathsf{A}_{\mathrm{eq}}^{-1}\Big] + \mathcal{O}(e^{-\mathsf{F}t}) \qquad (36)
\end{aligned}$$

Summing all the results so far, we can write the nonequilibrium heat generating function

as follows:

$$
\begin{aligned}
\mathcal{G}_\alpha(\lambda) = \frac{1}{(1-\lambda^2)^\nu}\exp\Bigg[ & \left(-\beta\lambda ku\left[\mathsf{F}^{-1}\cdot\mathbf{u}\right]_x + \beta(\lambda ku)^2[\mathsf{F}^{-1}\mathsf{A}_{\rm eq}^{-1}]_{xx}\right)\tau \\
& +\beta\lambda^3(ku)^2\Big[\underbrace{\underbrace{\int_0^\tau \mathrm{d}t e^{-\mathsf{F}t}\mathsf{A}_{\rm eq}^{-1}\mathsf{S}_\alpha^+(\mathsf{F}^{\rm t})^{-1}e^{-\mathsf{F}^{\rm t}t}}_{\mathsf{G}_\alpha^+} - \mathsf{F}^{-1}\mathsf{A}_{\rm eq}^{-1}\mathsf{S}_\alpha^+(\mathsf{F}^{\rm t})^{-1}}_{\delta G_\alpha^+}\Big]_{xx} \\
& +\beta\lambda^3(ku)^2\Big[\mathsf{A}_{\rm eq}^{-1}\underbrace{\Big(\underbrace{\int_0^\tau \mathrm{d}t e^{-\mathsf{F}^{\rm t}t}\mathsf{A}_{\rm eq}\mathsf{S}_\alpha^-\mathsf{F}^{-1}e^{-\mathsf{F}t}}_{\mathsf{G}_\alpha^-} - (\mathsf{F}^{\rm t})^{-1}\mathsf{A}_{\rm eq}\mathsf{S}_\alpha^-\mathsf{F}^{-1}\Big)\mathsf{A}_{\rm eq}^{-1}}_{\delta G_\alpha^-}\Big]_{xx} \\
& +\beta\lambda^3(ku)^2\Big[\mathsf{A}_{\rm eq}^{-1}(\mathsf{F}^{\rm t})^{-1}\mathsf{A}_{\rm eq}\mathsf{S}_\alpha^-\mathsf{F}^{-1}\mathsf{A}_{\rm eq}^{-1}\Big]_{xx} + \frac{(\beta\lambda)^2}{2}\mathbf{u}^{\rm t}\cdot(\mathsf{F}^{\rm t})^{-1}\mathsf{B}_\alpha\mathsf{S}_\alpha^-\mathsf{F}^{-1}\cdot\mathbf{u} \\
& -\beta\lambda^2 ku\ \left[\mathbf{u}^{\rm t}\cdot(\mathsf{F}^{-1})^{\rm t}\mathsf{B}_\alpha(\mathsf{I}-\lambda\mathsf{A}_{\rm eq}^{-1}\mathsf{B}_\alpha)^{-1}\mathsf{F}^{-1}\mathsf{A}_{\rm eq}^{-1}\right]_x \\
& +\frac{\beta\lambda}{2}\mathbf{u}^{\rm t}\cdot(\mathsf{F}^{\rm t})^{-1}\mathsf{B}_\alpha\mathsf{F}^{-1}\cdot\mathbf{u} + \beta\lambda ku\left[\mathsf{F}^{-2}\cdot\mathbf{u}\right]_x - \beta(\lambda ku)^2\mathsf{F}^{-2}[\mathsf{A}_{\rm eq}^{-1}]_{xx}\Bigg],
\end{aligned} \tag{37}
$$

which should be done more yet. The first line is proportional to $\tau$, which is the most dominant. The second line is proportional to $(1+\lambda)^{-1}$, which will contribute to the leading corrections to the large deviation function. The third line is proportional to $(1-\lambda)^{-1}$, but such singularity at $\lambda=-1$ is found to be cancelled by the next two lines. The final line is $\mathcal{O}(\tau^0)$.

$\mathsf{G}_\alpha^\pm$ or $\delta\mathsf{G}_\alpha^\pm$ cannot be evaluated directly from matrices. Integrating by parts and neglecting the upper limit$\sim e^{-\mathsf{F}\tau}$, we find

$$
G_\alpha^+ = \mathsf{F}^{-1}\mathsf{A}_{\rm eq}^{-1}\mathsf{S}_\alpha^+(\mathsf{F}^{\rm t})^{-1} - \mathsf{F}^{-1}\mathsf{G}_\alpha^+\mathsf{F}^{\rm t}, \tag{38}
$$

which gives

$$
\delta G_\alpha^+ + \mathsf{F}^{-1}\delta\mathsf{G}_\alpha^+\mathsf{F}^{\rm t} = -\mathsf{F}^{-2}\mathsf{A}_{\rm eq}^{-1}\mathsf{S}_\alpha^+ . \tag{39}
$$

Similarly, we find

$$
\delta G_\alpha^- + (\mathsf{F}^{\rm t})^{-1}\delta\mathsf{G}_\alpha^-\mathsf{F} = -(\mathsf{F}^{\rm t})^{-2}\mathsf{A}_{\rm eq}\mathsf{S}_\alpha^- . \tag{40}
$$

It is hardly possible to solve these matrix equations. By examining for $N=1,2,3$, we are able to conjecture the first matrix element of $\delta G_\alpha^+$. Writing

$$
[\delta G_\alpha^+]_{xx} = -\frac{N\gamma}{2k^2(1+\lambda)}b_\alpha \tag{41}
$$

we find

$$b_\alpha = \begin{cases} \frac{N\gamma}{k} + \frac{\mu}{N\gamma} & \text{for } \alpha = \mathrm{S} \\ \frac{(k+N\kappa)\gamma}{\kappa k} + \frac{\mu}{N\gamma} & \text{for } \alpha = \mathrm{B} \\ \frac{(k+N\kappa)\gamma}{\kappa k} + \frac{\mu+Nm}{N\gamma} & \text{for } \alpha = \mathrm{SB} \end{cases} . \tag{42}$$

We confirm numerically that the $(1-\lambda)^{-1}$ singularity from $\delta G_\alpha^-$ are cancelled by other lines in Eq. (29) for $N = 1, 2, 3$.

Using

$$[\mathsf{F}^{-1} \cdot \mathbf{u}]_x = \frac{N\gamma u}{k} \ , \quad [\mathsf{F}^{-1}\mathsf{A}^{\mathrm{eq}}]_{xx} = \cdot\mathbf{u}]_x = \frac{N\gamma}{k^2} \ , \tag{43}$$

we get

$$\mathcal{G}_\alpha(\lambda) = \frac{1}{(1-\lambda^2)^\nu} \exp\left[\tau N w(\lambda^2 - \lambda) - \frac{N w b_\alpha \lambda^3}{2(1+\lambda)} + \mathcal{O}(1)\right] \tag{44}$$

where $w = \langle \beta W \rangle/(N\tau) = \beta\gamma u^2$ is the dimensionless average work production rate per bath-particle for large $\tau$ limit.

## V. HEAT DISTRIBUTION FUNCTIONS FOR LONG TIME

### A. Equilibrium case

The equilibrium generating functions can be found by substituting $u = 0$ to Eq. (44), given as

$$\mathcal{G}_\alpha^{\mathrm{eq}}(\lambda) = \frac{1}{(1-\lambda^2)^\nu}. \tag{45}$$

Then, we find the equilibrium heat distribution for a dimensionless heat $r = \beta Q$ as

$$\begin{aligned} \mathcal{P}_\alpha^{\mathrm{eq}}(r) &= \int_{-\infty}^{\infty} \frac{\mathrm{d}\lambda}{2\pi} e^{i\lambda r} \mathcal{G}_\alpha^{\mathrm{eq}}(i\lambda) = \int_{-\infty}^{\infty} \frac{\mathrm{d}\lambda}{2\pi} \frac{e^{i\lambda r}}{(1+\lambda^2)^\nu} = \int_0^{\infty} \frac{\mathrm{d}\lambda}{\pi} \frac{\cos(\lambda r)}{(1+\lambda^2)^\nu} \\ &= \frac{(|r|/2)^{\nu-1/2}}{\sqrt{\pi}\Gamma(\nu)} K_{\nu-1/2}(|r|) \end{aligned} \tag{46}$$

where $K_\nu(z)$ is the second-kind modified Bessel function of order $\nu$. In particular, $\mathcal{P}_{\mathrm{S}}^{\mathrm{eq}}(r) = e^{-|r|}/2$, which interestingly is independent of $N$. The same result can be found for the equilibrium heat distribution for the single colloid in the Langevin dynamics in the large $\tau$ where the corresponding $\mathsf{F}$ matrix is give by $\begin{bmatrix} 0 & -1/m \\ k & \gamma/m \end{bmatrix}$. Difference of the two distributions lies in the transient period where $e^{-\mathsf{F}\tau}$ behaves differently for the two cases.

## B. nonequilibrium case

The nonequilibrium heat distribution function for $\beta Q = N\tau w q$ for large $\tau$ can be found form the Fourier transformation of Eq. (44), written as

$$\mathcal{P}_\alpha(q) = \int_{-i\infty}^{i\infty} \frac{\mathrm{d}\lambda}{2\pi i} \frac{1}{(1-\lambda^2)^\nu} \exp\left[\tau N w(\lambda^2 - \lambda + q\lambda) - \frac{N w b_\alpha \lambda^3}{2(1+\lambda)}\right] . \tag{47}$$

It can be evaluated by using the saddle-point approximation. which can be evaluated by using the saddle-point approximation in the large $\tau$ limit. Saddle point $\lambda^*$ is found from the extremum condition for the integrand of Eq. (47)

$$0 = \frac{\mathrm{d}}{\mathrm{d}\lambda}\left[\lambda^2 - \lambda - q\lambda + \frac{b_\alpha \lambda^3}{2\tau(1+\lambda)} - \frac{\nu}{N\tau w}\ln(1-\lambda^2)\right]_{\lambda=\lambda^*} \tag{48}$$

We find the heat distribution functions for three regions in $q$ below:

1. For $\lambda^*$ far from $\pm 1$ and $-1 < \lambda^* < 1$, the singular terms at $\lambda^* = \pm 1$ in Eq. (48) can be neglected, so $\lambda^* = (1-q)/2$ and $-1 < q < 3$. Expanding the integrand about the saddle point in Eq. (47) up to the second order in $x = \lambda - \lambda^*$,

$$\begin{aligned}\mathcal{P}_\alpha(q) &= \exp\left[-\tau N w \frac{(q-1)^2}{4}\right] \int_{-i\infty}^{i\infty} \frac{\mathrm{d}x}{2\pi i} \exp[\tau N w x^2] = \frac{1}{\sqrt{4\tau N w}} \exp\left[-\tau N w \frac{(q-1)^2}{4}\right] \\ &\simeq \exp\left[-\tau N w \frac{(q-1)^2}{4} - \frac{1}{2}\ln(\tau w)\right] , \quad \text{for } -1 < q < 3.\end{aligned} \tag{49}$$

2. For $\lambda^* \simeq 1$, we define $\delta\lambda_+ = \lambda^* - 1 < 0$. Then, the saddle-point condition leads to

$$1 - 2\lambda^* - q - \frac{\nu}{N\tau w}\frac{1}{1-\lambda^*} = 0 \;\text{ or }\; 2\delta\lambda_+ + (q+1) - \frac{\nu}{N\tau w}\frac{1}{\delta\lambda^+} = 0, \tag{50}$$

which gives

$$\delta\lambda_+ = \frac{1}{4}\left[-(q+1) - \sqrt{(q+1)^2 + \frac{8\nu}{N\tau w}}\right] , \tag{51}$$

for which there two cases: $(1+q)^2 \gg \frac{8\nu}{N\tau w}$ and $(1+q)^2 \ll \frac{8\nu}{N\tau w}$. The latter is restricted to a very narrow region, so we only consider the former case with

$$\delta\lambda_+ \simeq -\frac{4\nu}{N\tau w |q+1|} , \quad \text{for } q < -1 . \tag{52}$$

The usual saddle-point approximation cannot be used because $(1-\lambda^2)^{-\nu}$ in the integrand cannot be expanded about $\lambda^* \simeq 1$. We use a new variable $v$ such that

$$(1-\lambda)^{-1} = [1 - \lambda^* - (\lambda - \lambda^*)]^{-1} = (-\delta\lambda_+)^{-1}\left(1 + \frac{\lambda - \lambda^*}{\delta\lambda_+}\right)^{-1} = \frac{1}{(-\delta\lambda_+)v} , \tag{53}$$

which is treated exactly. Expanding other terms about $\lambda = \lambda^*$ and using $\lambda - \lambda^* = \delta\lambda_+(v-1)$ and $\lambda^* = 1 + \delta\lambda_+$, we can get

$$\begin{aligned}
\mathcal{P}_\alpha(q) &\simeq -\frac{1}{|\delta\lambda_+|^{\nu-1}} \int_{1-i\infty}^{1+i\infty} \frac{dv}{2\pi i} \frac{e^{\tau N w(q+(q+1)v\delta\lambda^+ + (\delta\lambda^+)^2 v^2)}}{(-2^\nu)v^\nu} \\
&\simeq \frac{e^{\tau N w q}}{|\delta\lambda_+|^{\nu-1}(-2^\nu)} \underbrace{\int_{1-i\infty}^{1+i\infty} \frac{dv}{2\pi i} \frac{e^{4\nu v}}{v^\nu}}_{\mathcal{O}(1)} \\
&\simeq \exp\left[\tau N w q + (\nu - 1)\ln(w\tau)\right] \qquad (54)
\end{aligned}$$

3. For $\lambda^* \simeq -1$, we can neglect the terms with $1-\lambda$. Defining $\delta\lambda_- = \lambda^* + 1 > 0$, the saddle point equation is given as

$$1 - 2\lambda^* - q + \frac{b_\alpha}{2\tau(1+\lambda^*)^2} = 0 \ , \quad \text{or} \quad -2\delta\lambda^- - (q-3) + \frac{b_\alpha}{2\tau(\delta\lambda_-)^2} = 0 \ . \qquad (55)$$

We omit the narrow region for $q - 3 \ll \delta\lambda_-$. For $q - 3 \gg \delta\lambda_-$, we get

$$\delta\lambda_- = \left[\frac{b_\alpha}{2\tau(q-3)}\right]^{1/2} \ , \quad \text{for } p - 3 \gg \left[\frac{b_\alpha}{2\tau}\right]^{1/3} . \qquad (56)$$

Similarly to the case for $q < -1$, we write $(1+\lambda)^{-1} = (\delta\lambda_+ u)^{-1}$ using a new variable $u$. We treat $(1+\lambda)^{-1}$ exactly and expand other terms of the integrand in Eq. (47) up to $(\lambda - \lambda^*)^2$ order, we find

$$\mathcal{P}_\alpha(q) \simeq \frac{e^{-\tau N w(p-2)}}{(\delta\lambda_-)^{\nu-1} 2^\nu} \int_{1-i\infty}^{1+i\infty} \frac{du}{2\pi i} \frac{1}{u^\nu} \exp\left[Nw\sqrt{\frac{\tau(q-3)}{2}}\left(u + \frac{1}{u}\right)\right] \ . \qquad (57)$$

The integral over $u$ can be found by using the saddle-point approximation for the saddle point $u^* = 1$ given from $\mathrm{d}(u + 1/u)/\mathrm{d}u|_{u=u^*} = 0$. Then, we find

$$\begin{aligned}
\mathcal{P}_\alpha(q) &\simeq \frac{e^{-\tau N w(p-2) + Nw\sqrt{2\tau(q-3)b_\alpha}}}{(\delta\lambda_-)^{\nu-1} 2^\nu} \int_{1-i\infty}^{1+i\infty} \frac{du}{2\pi i} \exp\left[Nw\sqrt{\frac{\tau(p-3)b_\alpha}{2}}(u-1)^2\right] \\
&\simeq \left[\frac{2\tau(q-3)}{b_\alpha}\right]^{\frac{\nu-1}{2}} \frac{e^{-\tau N w(p-2) + Nw\sqrt{2\tau(q-3)b_\alpha}}}{[Nw[\tau(q-3)b_\alpha/2]^{1/2}]^{1/2}} \\
&\simeq \exp\left[-\tau N w(p-2) + N\sqrt{2\tau w^2(q-3)b_\alpha} + \left(\frac{\nu}{2} - \frac{3}{4}\right)\ln(\tau w^2(q-3)b_\alpha)\right] \qquad (58)
\end{aligned}$$
